# Supplementary material for: Reaction-transport coupling drives spatiotemporal organization in fuel-driven supramolecular polymerization
Source: arXiv:2601.15662 ancillary file (2026-05-28)
Supplement: Supplementary file 1 [file Supporting_Info.pdf]

# Supporting Information

## “Emergence of spatiotemporal patterns in a fuel-driven coupled cooperative supramolecular system”

Akta Singh<sup>a</sup>, Nayana Mukherjee<sup>b</sup>, Jagannath Mondal <sup>\*a</sup>, and Pushpita Ghosh <sup>†c</sup>

<sup>a</sup>Tata Institute of Fundamental Research Hyderabad, Telangana 500046, India

<sup>b</sup>Department of Mathematics. Mahindra University, Hyderabad, Telangana 500043, India

<sup>c</sup>School of Chemistry, Indian Institute of Science Education and Research,  
Thiruvananthapuram, Kerala 695551, India

---

### Contents

|          |                                                  |            |
|----------|--------------------------------------------------|------------|
| <b>1</b> | <b>Linear Stability Analysis</b>                 | <b>S-2</b> |
| <b>2</b> | <b>Numerical Integration</b>                     | <b>S-3</b> |
| 2.1      | Temporal system . . . . .                        | S-3        |
| 2.2      | Reaction–diffusion system . . . . .              | S-3        |
| <b>3</b> | <b>Movies</b>                                    | <b>S-4</b> |
| 3.1      | Movie-S1 . . . . .                               | S-4        |
| 3.2      | Movie-S2 . . . . .                               | S-4        |
| 3.3      | Movie-S3 . . . . .                               | S-4        |
| <b>4</b> | <b>Calculating the wavefront spread</b>          | <b>S-4</b> |
| <b>5</b> | <b>Effect of system size and grid resolution</b> | <b>S-4</b> |
| <b>6</b> | <b>Figures</b>                                   | <b>S-5</b> |

---

\*jmondal@tifrh.res.in

†pushpita@iisertvm.ac.in

# 1 Linear Stability Analysis

To analyze the conditions under which the spatially homogeneous steady state of the system becomes unstable to spatial or spatiotemporal perturbations, we perform a linear stability analysis of the system described by the temporal kinetic equations. The full four-variable model presented in Eqs. (1)–(4) of the main text can be reduced to an equivalent three-component system by invoking the conservation constraint

$$c_{\text{tot}} = d + a_1 + m'_1, \quad (1)$$

which allows us to eliminate one variable without loss of generality. Substituting this constraint into the governing equations yields a closed system of three coupled equations of the form

$$\dot{a}_1 = k'_a(c_{\text{tot}} - a_1 - m'_1) - 2k_+a_1m'_0 \quad (2)$$

$$\dot{m}'_1 = -2k'_{d2}m'_0 + 2k_+a_1m'_0 \quad (3)$$

$$\dot{m}'_0 = k'_{d3}(m'_1 - 4m'_0) - \frac{2k'_{d2}Cm'_0}{(m'_1/m'_0 - 2)^2} - 2k'_{d3}m'_0 - k_+(m'_0)^2 \quad (4)$$

Let  $(a_1^*, m_1^*, m_0^*)$  denote the homogeneous steady state obtained by solving  $\dot{a}_1 = \dot{m}'_1 = \dot{m}'_0 = 0$ . To assess its stability, we evaluate the Jacobian matrix  $J$  of the system at this steady state [Strogatz(2018)]. Introducing an infinitesimal perturbation  $\delta \mathbf{x} = (\delta a_1, \delta m'_1, \delta m'_0)^T$ , the linearized dynamics is governed by

$$\frac{d}{dt} \delta \mathbf{x} = J \delta \mathbf{x}. \quad (5)$$

A solution of this system takes the form  $\delta \mathbf{x}(t) = \mathbf{v} e^{\lambda t}$ , where  $\lambda$  and  $\mathbf{v}$  are the eigenvalue and eigenvector of  $J$ , respectively. Substituting this ansatz into the linearized equation yields the standard eigenvalue problem

$$(J - \lambda I) \mathbf{v} = 0, \quad (6)$$

which in turn leads to the characteristic equation

$$\det(J - \lambda I) = 0. \quad (7)$$

The characteristic equation (7) for this three-component kinetic system yields a cubic polynomial in  $\lambda$  of the general form

$$\lambda^3 - s_1 \lambda^2 + s_2 \lambda - s_3 = 0, \quad (8)$$

where the coefficients  $s_1$ ,  $s_2$ , and  $s_3$  are determined by the trace, principal minors, and determinant of the Jacobian matrix  $J$ . These coefficients encode the local dynamical behavior of the system near the homogeneous steady state. The three eigenvalues  $\lambda_1, \lambda_2, \lambda_3$  are obtained as the roots of Eq. (8).

Analytically solving the cubic equation is possible in principle, but the resulting expressions are unwieldy and offer limited physical insight for the nonlinear reaction kinetics under study. Therefore, in practice, we compute the eigenvalues numerically by directly evaluating the full Jacobian matrix at the steady state. This approach allows us to efficiently determine whether the real parts of the eigenvalues change sign as parameters vary. In particular, the transition to oscillatory behavior is identified when a pair of complex conjugate eigenvalues crosses the imaginary axis, signaling a Hopf bifurcation, while purely real eigenvalue crossings indicate non-oscillatory instabilities.

## Numerical procedure:

For a fixed set of kinetic parameters  $(k'_a, k'_{d2}, k'_{d3})$ , the linear stability of the homogeneous steady state is determined using the following steps:

1. **Steady-state computation.** The homogeneous steady state  $(a^*, m_1^*, m_0^*)$  is obtained by solving the system of nonlinear algebraic equations

$$\dot{a}_1 = 0, \quad \dot{m}'_1 = 0, \quad \dot{m}'_0 = 0,$$

where the time derivatives are given by Eqs. (2)–(4).

2. **Jacobian evaluation.** The Jacobian matrix  $J$  is evaluated at the steady state using the explicit partial derivatives of Eqs. (2)–(4). Fixing  $C = 4.6$ , the Jacobian takes the form

$$J(a^*, m_1^*, m_0^*) = \begin{pmatrix} -2k_+m_0^* - k'_a & -k'_a & -2k_+a^* \\ 2k_+m_0^* & 0 & 2k_+a^* - 2k'_{d2} \\ 0 & \frac{18.4k'_{d2}m_0^{*3}}{(m_1^* - 2m_0^*)^3} + k'_{d3} & -2k_+m_0^* - \frac{9.2k'_{d2}m_0^{*2}}{(m_1^* - 2m_0^*)^2} - \frac{18.4k'_{d2}m_1^*m_0^{*2}}{(m_1^* - 2m_0^*)^3} - 6k'_{d3} \end{pmatrix}.$$

3. **Eigenvalue computation.** The eigenvalues of  $J$  are obtained numerically:

$$\lambda_i = \text{eig}(J), \quad i = 1, 2, 3.$$

The sign of  $\text{Re}(\lambda_i)$  determines the stability of the steady state, while a complex-conjugate pair crossing the imaginary axis identifies a Hopf bifurcation.

**Stability criterion:** The linear stability of the homogeneous steady state is determined by the real parts of the eigenvalues of the Jacobian matrix:

- If  $\Re(\lambda_i) < 0$  for all  $i$ , the steady state is *linearly stable*, and all small perturbations decay exponentially in time.
- If any  $\Re(\lambda_i) > 0$ , the steady state is *unstable*, and perturbations grow with time.

In particular, the emergence of a complex-conjugate pair of eigenvalues crossing the imaginary axis (i.e.,  $\Re(\lambda) = 0$  with  $\Im(\lambda) \neq 0$ ) signals a Hopf bifurcation, marking the onset of sustained oscillations in the temporal dynamics.

## 2 Numerical Integration

### 2.1 Temporal system

We numerically integrate the full temporal reaction kinetics given in Eqs. (1)–(4) of the main text to characterize the dynamical behavior across the parameter space in both the stable and oscillatory regimes. To probe the response of the system to small disturbances, the integration is initialized at the homogeneous steady state with an added infinitesimal perturbation applied to each variable.

The temporal evolution is computed using a forward Euler scheme with a timestep  $\Delta t = 10^{-4}$  and a total integration time of  $t_{\text{max}} = 100$  (dimensionless units). This choice of timestep ensures numerical stability while accurately resolving the oscillatory dynamics near the Hopf bifurcation. For each parameter set, we monitor the time series of  $a_1(t)$ ,  $m'_1(t)$ , and  $m'_0(t)$  to determine whether perturbations decay (stable steady state) or grow into sustained oscillations (limit cycle behavior).

### 2.2 Reaction–diffusion system

To simulate the system in two spatial dimensions, the reaction model is extended by incorporating diffusion terms (Eqs. 5–8 of the main text). Following the Rouse scaling, the polymer diffusion coefficient depends on its instantaneous average length,

$$L_p = \frac{m'_1}{m'_0},$$

such that

$$D_m = \frac{D_0}{L_p}.$$

The monomer diffusion coefficient is fixed at  $D_0 = 1$  in dimensionless units.

The reaction–diffusion equations are solved numerically on a two-dimensional  $100 \times 100$  grid using an explicit Euler forward scheme with time step  $\Delta t = 10^{-4}$  and spatial discretization  $\Delta x = \Delta y = 0.5$ . Zero-flux

(Neumann) boundary conditions are imposed on all sides. Each grid point is initialized with the homogeneous steady-state values of the four variables  $(d, a_1, m'_1, m'_0)$ , and the initial symmetry is broken by adding random perturbations of amplitude  $10^{-2}$  drawn from a uniform distribution. At each time step, the local polymer length  $L_p$  is computed and used to update the local diffusion coefficient  $D_m$ .

To study traveling-wave dynamics in greater detail, we later introduce a localized Gaussian perturbation to the polymer mass concentration  $m'_1$  and the polymer number concentration  $m'_0$  at the center of the spatial domain, while maintaining steady-state values for all four fields elsewhere.

### 3 Movies

#### 3.1 Movie-S1

*Movie-S1*: Spatiotemporal evolution of reaction-diffusion system with perturbation drawn from uniform random distribution (parameter set  $k'_a = 4$ ,  $k'_{d2} = 5000$ , and  $k'_{d3} = 1.5$ ).

#### 3.2 Movie-S2

*Movie-S2*: Spatiotemporal evolution of reaction-diffusion system with Gaussian perturbation at domain center (parameter set  $k'_a = 4$ ,  $k'_{d2} = 5000$ , and  $k'_{d3} = 1.5$ ).

#### 3.3 Movie-S3

*Movie-S3*: Spatiotemporal evolution of reaction-diffusion system with Gaussian perturbation at domain center (parameter set  $k'_a = 0.9$ ,  $k'_{d2} = 2000$ , and  $k'_{d3} = 0.1$ ).

## 4 Calculating the wavefront spread

To quantify the propagation of the wavefront, we compute the gradient field of the polymer mass concentration,

$$g = |\nabla m'_1|,$$

evaluated at every spatial point and at each timestep. The spatial spread of this gradient field is measured by tracking the interface positions along the  $x$ - and  $y$ -directions, defined respectively as

$$X^2 = \frac{\int x^2 g(x, y) dx dy}{\int g(x, y) dx dy}, \quad Y^2 = \frac{\int y^2 g(x, y) dx dy}{\int g(x, y) dx dy}.$$

The overall root-mean-square spatial spread is then computed as

$$R = \sqrt{X^2 + Y^2}.$$

We evaluate  $R(t)$  as a function of time and analyze its temporal scaling. On a log-log scale, the resulting data are fit to a power-law relation, enabling extraction of the corresponding scaling exponent that characterizes the spreading dynamics of the wavefront.

## 5 Effect of system size and grid resolution

To assess the robustness of the observed reaction–diffusion dynamics, we examined the influence of both the system size and the spatial grid resolution on the emergence and evolution of spatiotemporal patterns. These tests ensure that the reported behaviors are intrinsic to the model dynamics and not artifacts of finite-size effects or numerical discretization.

To probe finite-size effects, the spatial domain was increased from  $100 \times 100$  to  $200 \times 200$  grid points while keeping the spatial resolution fixed at  $\Delta x = \Delta y = 0.5$ . All other parameters, including kinetic rate constants, time step, boundary conditions, and initialization procedure, were kept identical. Increasing the

domain size allows a larger number of supramolecular polymer seeds to form under random perturbations, which subsequently evolve into multiple spreading wavefronts (Fig. S2). For simulations initialized with Gaussian perturbations, the larger domain permits the wavefront to propagate for a longer duration before interacting with the system boundaries and ultimately collapsing (Fig. S3). Aside from these finite-size effects, no significant qualitative changes in the spatiotemporal dynamics were observed.

To examine the role of numerical resolution, simulations were performed at two different spatial grid spacings,  $\Delta x = \Delta y = 0.5$  and  $\Delta x = \Delta y = 0.1$ , while keeping the overall domain size fixed at  $100 \times 100$ . All remaining parameters were unchanged. For Gaussian perturbations, increasing the spatial resolution results in smoother and more isotropic wavefronts, yielding a more circular propagation profile (Fig. S4). We furthermore examine the effect of spatial grid resolution using a nine-point stencil discretization and it shows prolonged circularly propagating wave fronts before it breaks the symmetry as shown in Fig. S5. Importantly, the qualitative features of the dynamics, including wavefront initiation, propagation, and decay, remain robust across grid resolutions, indicating that the observed patterns are not numerical artifacts.

## 6 Figures

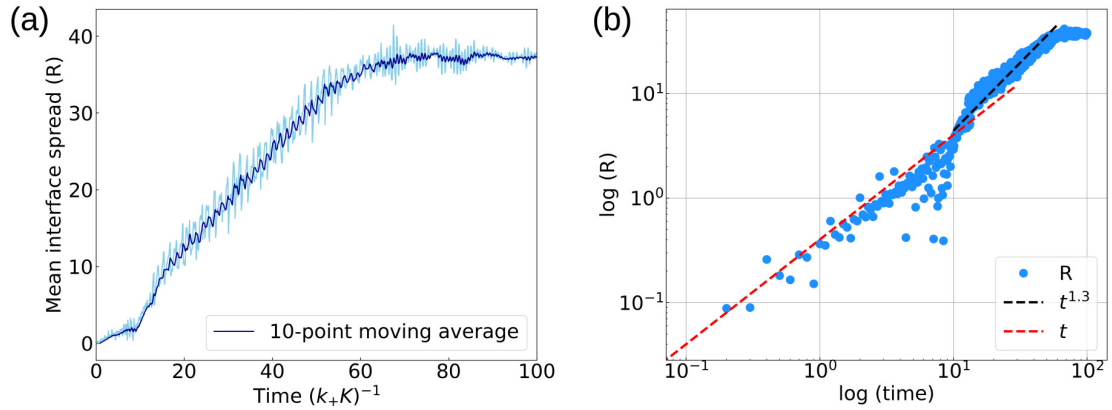

**Figure S1:** (a) Temporal evolution of the interface spread for a Gaussian-perturbed system near the bifurcation surface ( $k'_a = 0.9$ ,  $k'_{d2} = 2000.0$ , and  $k'_{d3} = 0.1$ ). (b) Power-law scaling of the interface spread with time for the same parameter set, showing two distinct regimes: linear and accelerated growth.

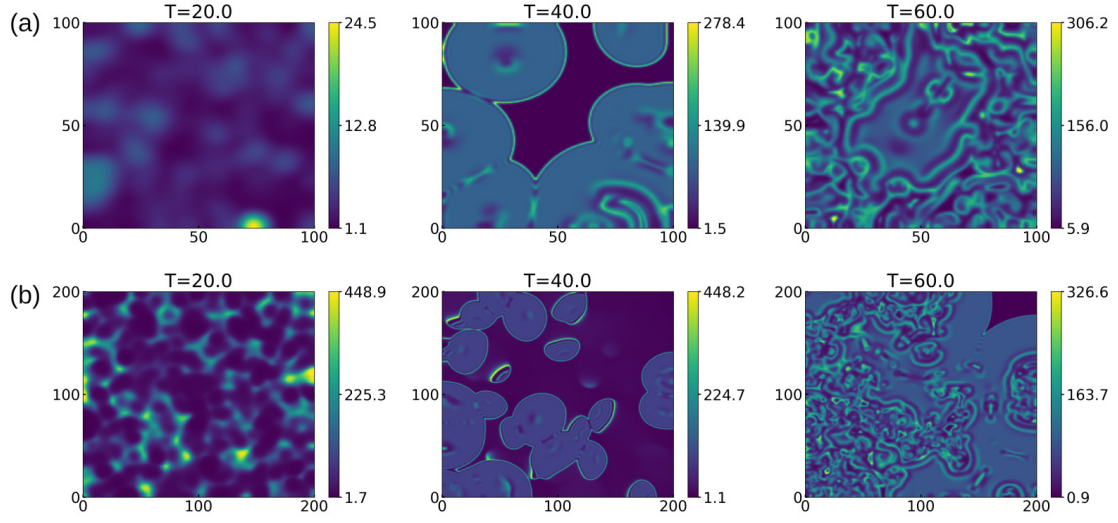

**Figure S2:** Effect of system size. Snapshots of polymer mass concentration evolution for domain size (a)  $100 \times 100$  and (b)  $200 \times 200$  at different time using random perturbation from uniform distribution (parameter set  $k'_a = 4$ ,  $k'_{d2} = 5000$ , and  $k'_{d3} = 1.5$ ). Grid size is 0.5. Time is in unit  $(k_+ K)^{-1}$ .

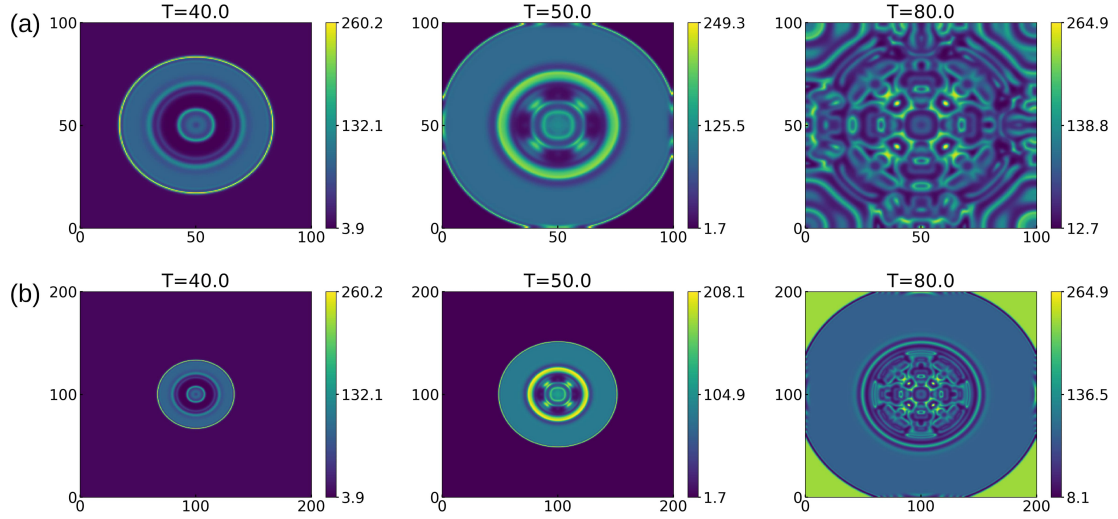

**Figure S3:** Effect of system size. Snapshots of polymer mass concentration evolution for domain size (a)  $100 \times 100$  and (b)  $200 \times 200$  at different time using Gaussian perturbation (parameter set  $k'_a = 4$ ,  $k'_{d2} = 5000$ , and  $k'_{d3} = 1.5$ ). Grid size is 0.5. Time is in unit  $(k_+ K)^{-1}$ .

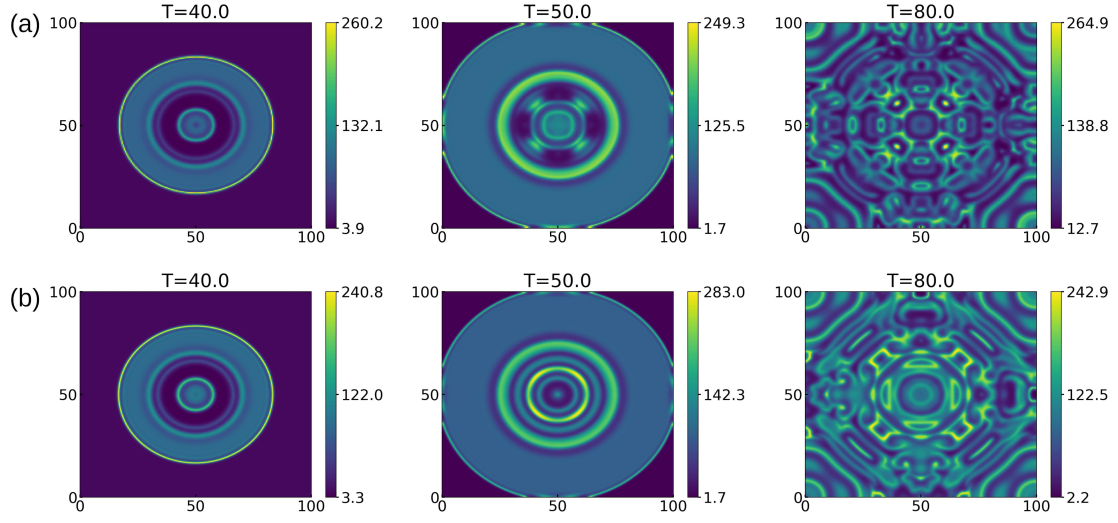

**Figure S4:** Effect of grid size. Snapshots of polymer mass concentration evolution for grid size (a) 0.5 and (b) 0.1 at different time using Gaussian perturbation (parameter set  $k'_a = 4$ ,  $k'_{d2} = 5000$ , and  $k'_{d3} = 1.5$ ). Domain size is  $100 \times 100$ . Time is in unit  $(k_+K)^{-1}$ .

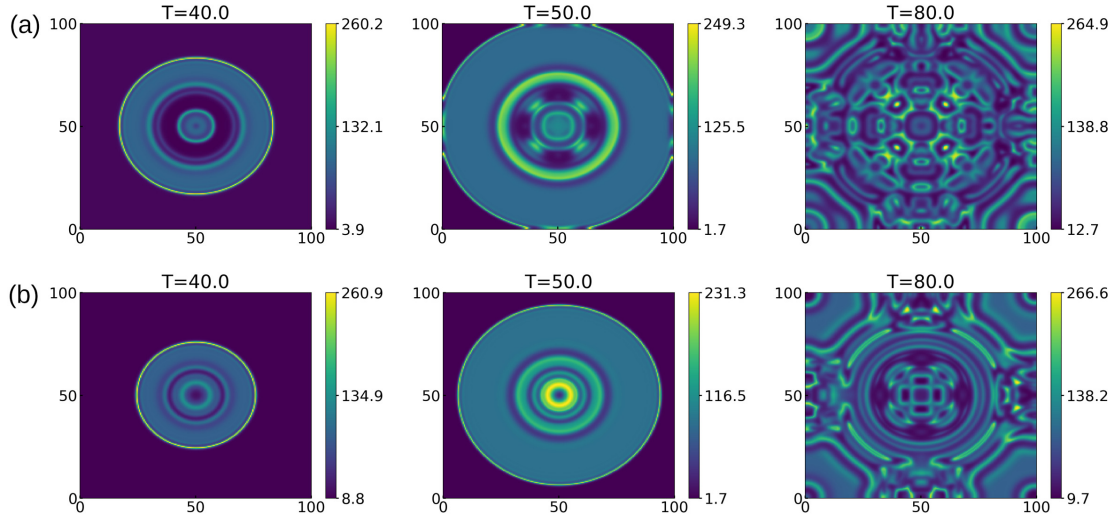

**Figure S5:** Comparison between snapshots of polymer mass concentration evolution for domain size  $100 \times 100$  and grid size 0.5 with (a) 5-point finite difference and (b) 9-point finite difference scheme at different times using Gaussian perturbation (parameter set  $k'_a = 4$ ,  $k'_{d2} = 5000$ , and  $k'_{d3} = 1.5$ ). Time is in unit  $(k_+K)^{-1}$ .

## References

[Strogatz(2018)] S. H. Strogatz, *Nonlinear Dynamics and Chaos: With Applications to Physics, Biology, Chemistry, and Engineering*, CRC Press, Boca Raton, FL, 2nd edn., 2018.
